# Supplementary material for: Integrated Digital Image Correlation for Micro-Mechanical Parameter Identification in Multiscale Experiments
Source: arXiv:2302.03600 source file (2023-02-03)

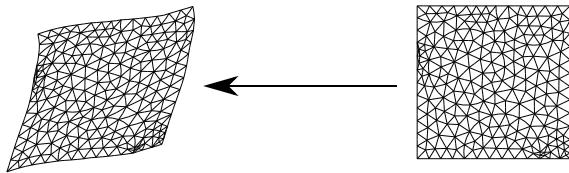

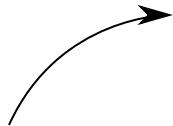

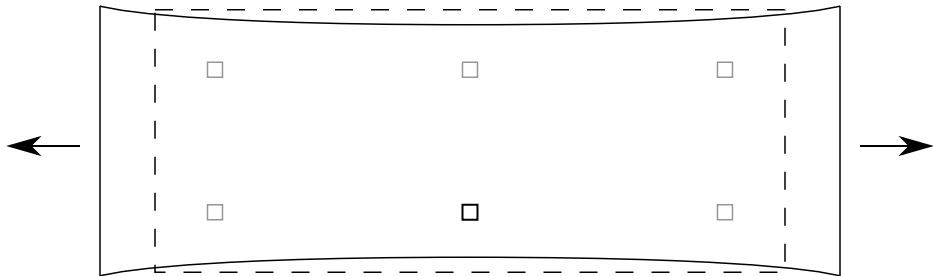

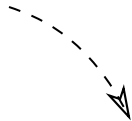

Supplement: Supplementary file 2 [file sketch_SI_ink.pdf]
